# Supplementary material for: MolLangData: A Large-Scale Dataset for Molecular Structure-Language Description via a Rule-Regularized Method
Source: arXiv:2602.02320 source file (2026-09-26)
Supplement: Supplementary file 1 [file representative_error_examples.tex]

\subsection{Representative Error Samples}
\label{sec:error_samples}
